# Supplementary material for: Berserker: ASN.1-based Fuzzing of Radio Resource Control Protocol for 4G and 5G
Source: arXiv:2107.01912 source file (2021-12-02)
Supplement: Supplementary file 1 [file chapter07_appendix_a.tex]

\subsection*{Results from Generation-based Fuzzing} \label{appendix_B}
% todo - add labels for dl as well
This appendix provides experimental results when Berserker used generation-based fuzzing to replace various RRC messages as shown in Tables \ref{tab:results_generation_strategies_con_req} - \ref{tab:results_generation_strategies_ue_cap_enq}. Each table corresponds to the RRC message's PDU that Berserker replaces with RRC PDU*. For every message, we identify the possible mutations on ASN.1 schema following Table \ref{tab:mutation_strategies_asn1}. The tables contain number of RRC PDUs replaced, time taken to conduct the tests, time taken between receiving a RRC PDU and producing a RRC PDU* by RRC message generator, and the initial seeds we used to control the experiments. In addition to mutating ASN.1 schemas, we send other RRC messages that are generated using original ASN.1 schema during perturbation.
